# Supplementary material for: M2Lens: Visualizing and Explaining Multimodal Models for Sentiment Analysis
Source: arXiv:2107.08264 source file (2021-08-29)
Supplement: Supplementary file 1 [file supplementary.tex]

\section{Supplementary Material}

\subsection{Multimodal Feature Sets}

\subsubsection{Language Feature Sets} 
\begin{itemize}
\item \textit{POS tags}: [ADJ, ADP, ADV, AUX, CONJ, CCONJ, DET, INTJ, DET, INTJ, NOUN, NUM, PART, PRON, PROPN, PUNCT, SCONJ, SYM, VERB, X]
\end{itemize}

\subsubsection{Audio Feature Sets}
\begin{itemize}
\item \textit{Pitch}:[F0]
\item \textit{Glottal}:[VUV, NAQ, QOQ, H1H2, PSP, MDQ, peakSlope, Rd, Rd\_conf, creak]
\item \textit{Amplitude}:[MCEP\_0, MCEP\_1, MCEP\_2, MCEP\_3, MCEP\_4, MCEP\_5, MCEP\_6, MCEP\_7, MCEP\_8, MCEP\_9, MCEP\_10, MCEP\_11, MCEP\_12, MCEP\_13, MCEP\_14, MCEP\_15, MCEP\_16, MCEP\_17, MCEP\_18, MCEP\_19, MCEP\_20, MCEP\_21, MCEP\_22, MCEP\_23, MCEP\_24]
\item \textit{Phase}:[HMPDM\_0, HMPDM\_1, HMPDM\_2, HMPDM\_3, HMPDM\_4, HMPDM\_5, HMPDM\_6, HMPDM\_7, HMPDM\_8, HMPDM\_9, HMPDM\_10, HMPDM\_11, HMPDM\_12, HMPDM\_13, HMPDM\_14, HMPDM\_15, HMPDM\_16, HMPDM\_17, HMPDM\_18, HMPDM\_19, HMPDM\_20, HMPDM\_21, HMPDM\_22, HMPDM\_23, HMPDM\_24, HMPDD\_0, HMPDD\_1, HMPDD\_2, HMPDD\_3, HMPDD\_4, HMPDD\_5, HMPDD\_6, HMPDD\_7, HMPDD\_8, HMPDD\_9, HMPDD\_10, HMPDD\_11, HMPDD\_12]
\end{itemize}

\subsubsection{Vision Feature Sets}
\begin{itemize}
\item \textit{Face emotion}: [Anger, Contempt, Disgust, Joy, Fear, Baseline, Sadness, Surprise, Confusion, Frustration]
\item \textit{Brow}: [AU1, AU2, AU4]
\item \textit{Eye}: [AU5, AU6, AU7, AU43]
\item \textit{Nose}: [AU9]
\item \textit{Lip}: [AU10, AU12, AU14, AU15,AU18, AU20, AU23, AU24, AU25, AU28],
\item \textit{Chin}: [AU17,AU26]
\item \textit{Head movement}:[Pitch, Yaw, Roll]
\item \textit{Others}: [Has\_Glasses, Is\_Male]
\end{itemize}

Below are the descriptions for corresponding facial action units:
\begin{compactitem}
\item \textit{AU1}: Inner Brow Raiser
\item \textit{AU2}: Outer Brow Raiser
\item \textit{AU4}: Brow Lowerer
\item \textit{AU5}: Upper Lid Raiser
\item \textit{AU6}: Cheek Raiser
\item \textit{AU7}: Lid Tightener
\item \textit{AU9}: Nose Wrinkler
\item \textit{AU10}: Upper Lip Raiser
\item \textit{AU12}: Lip Corner Puller
\item \textit{AU14}: Dimpler
\item \textit{AU15}: Lip Corner Depressor
\item \textit{AU16}: Lower Lip Depressor
\item \textit{AU17}: Chin Raiser
\item \textit{AU18}: Lip Puckerer
\item \textit{AU20}: Lip Stretcher
\item \textit{AU23}: Lip Tightener
\item \textit{AU24}: Lip Pressor
\item \textit{AU25}: Lips part
\item \textit{AU26}: Jaw Drop
\item \textit{AU28}: Lip Suck
\item \textit{AU43}: Eyes Closed
\item \textit{Anger}: Brow Lowerer, Upper Lid Raiser, Lid Tightener, Lip Tightener
\item \textit{Contempt}: Lip Corner Puller, Dimpler
\item \textit{Disgust}: Nose Wrinkler, Lip Corner Depressor, Lower Lip Depressor
\item \textit{Joy}: Cheek Raiser, Lip Corner Puller
\item \textit{Fear}: Inner Brow Raiser, Outer Brow Raiser, Brow Lowerer, Upper Lid Raiser,Lid Tightener, Lip Stretcher, Jaw Drop
\item \textit{Sadness}: Inner Brow Raiser, Brow Lowerer, Lip Corner Depressor
\item \textit{Surprise}: Inner Brow Raiser, Outer Brow Raiser, Upper Lid Raiser, Jaw Drop
\item \textit{Baseline, Confusion, and Frustration}: No Description Info
% \item Confusion]: No Description Info
% \item Frustration]: No Description Info
\end{compactitem}

\subsection{Models}
\begin{figure}[htb]
\centering 
\includegraphics[width=0.5\textwidth]{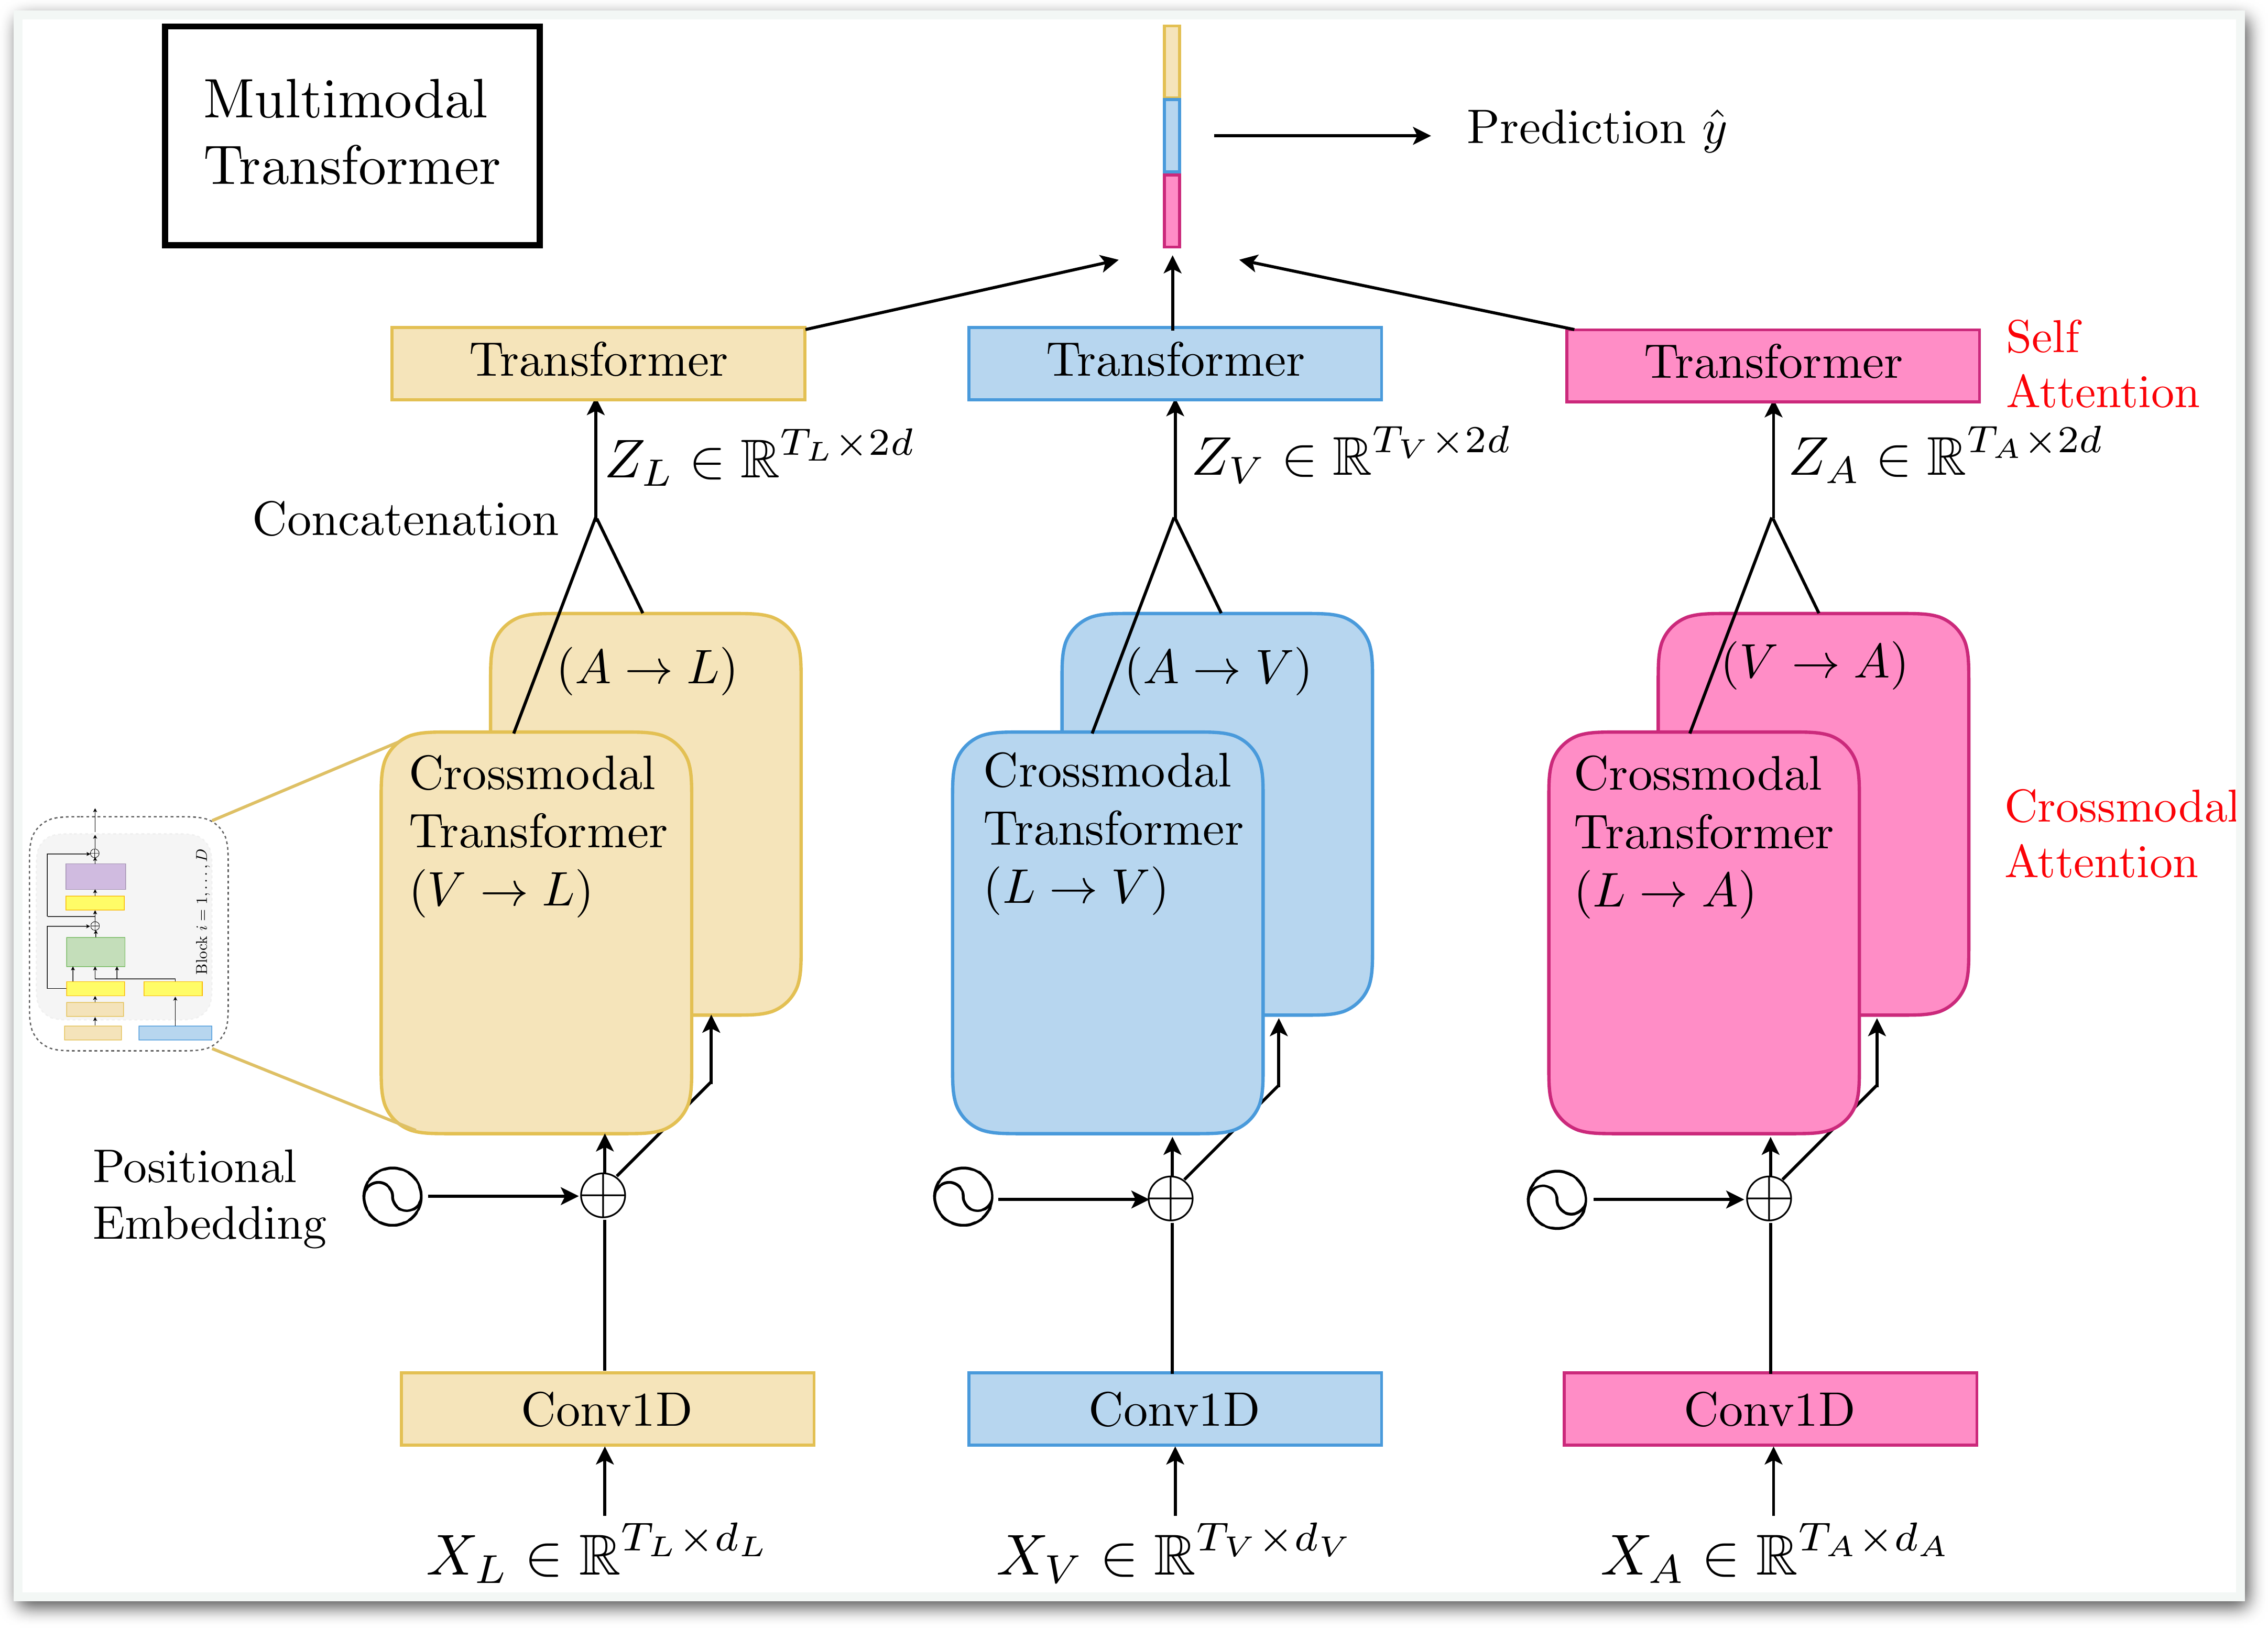}
\vspace{-5mm}
\caption{
Model Architecture for Multimodal Transformer (MulT).
} 
\label{fig.mult}
\end{figure}

\begin{figure}[htb]
\centering 
\includegraphics[width=0.5\textwidth]{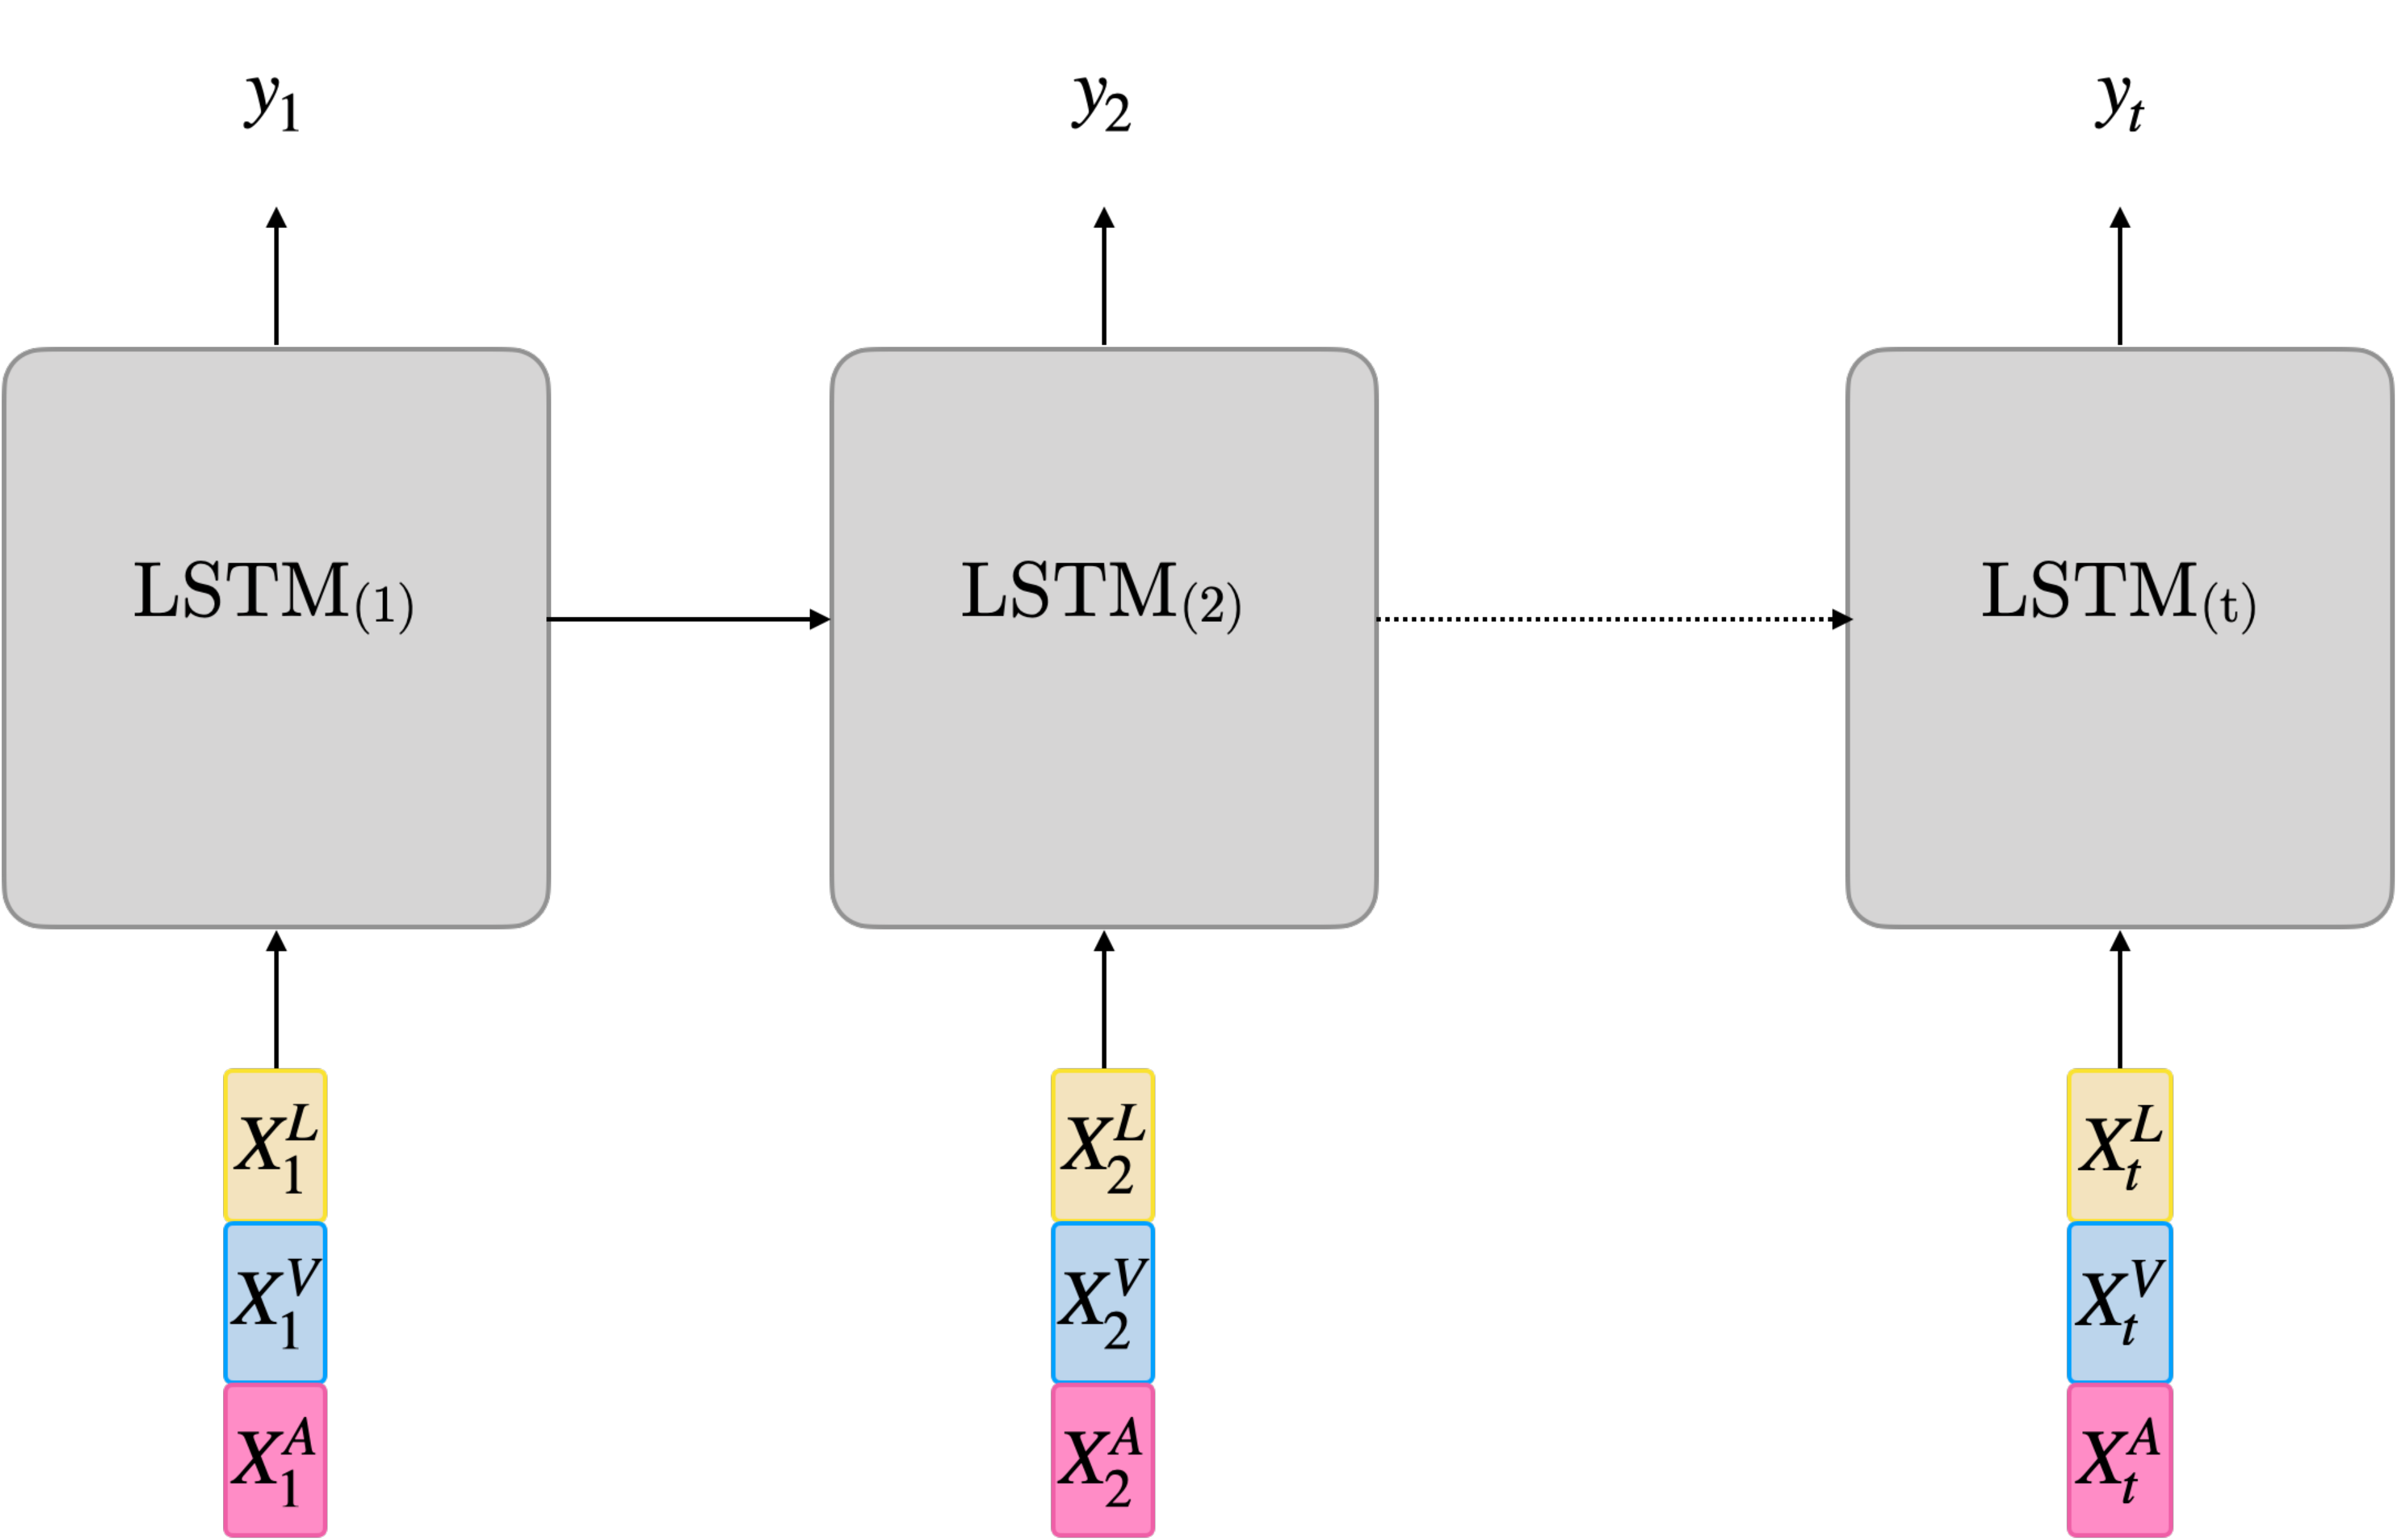}
\vspace{-5mm}
\caption{
Model Architecture for Early fusion LSTM (EF-LSTM).
} 
\label{fig.ef-lstm}
\end{figure}

We demonstrate the model architectures for Multimodal Transformer (MulT)~\cite{tsai2019multimodal} in Fig. \ref{fig.mult} and early fusion LSTM (EF-LSTM) in Fig. \ref{fig.ef-lstm}. In MulT, there are multiple crossmodal transformers which learn to transform the low-level features to one modality to the target modality. After that, it learns to model the concatenated results from cross model transformer using self-attention and output the prediction. In EF-LSTM, features from three modalities are simply concatenated (or fused) before input to the LSTM cell, and the LSTM cell produces one prediction at each time step. For both figures, we use $X_L, X_V, X_A$ to represent the input features and $y$ as the predictions, where $L, V, A$ indicate the language, visual and acoustic modalities respectively. For MulT, $T$ and $d$ are used to represent the sequence length and feature dimension of the corresponding modality. $Z$ indicates the concatenated output of two crossmodal transformers with the same target modality.
